# Supplementary material for: Predicting the State of Synchronization of Financial Time Series using Cross Recurrence Plots
Source: arXiv:2210.14605 source file (2022-11-02)
Supplement: Supplementary file 1 [file Appendix.tex]

\begin{small}
\begin{longtable}[h]{llcccccc}
\caption{Performance on the test set for all the stock pairs in Table~\ref{tb:data}. \enquote{Pct. class 1} refers to the fraction of targets in class 1 (time-series synchronization), \enquote{$w^\star$} is the value of the hyperparameter $w$ under which the best F1-score is observed. Results refer to the 3-dimensional times series consisting of prices, volumes and returns.}\\
\toprule
Stock Pair & Sector & F1-score & Accuracy & Precision & Recall & \multicolumn{1}{l}{Pct. Class 1} & $w^\star$ \\
\midrule
CVX - HD & EM - RT & 0.86  & 0.91  & 0.86  & 0.86  & 0.79  & 20 \\
WMT - GOOG & TS - EM & 0.85  & 0.86  & 0.85  & 0.86  & 0.40  & 20 \\
CVX - MSFT & EM - RT & 0.84  & 0.88  & 0.83  & 0.87  & 0.75  & 20 \\
XOM - JPM & TS - RT & 0.84  & 0.85  & 0.83  & 0.85  & 0.35  & 20 \\
CVX - GOOG & EM    & 0.84  & 0.87  & 0.83  & 0.85  & 0.74  & 20 \\
QCOM - CVX & ET - EM & 0.82  & 0.83  & 0.83  & 0.82  & 0.56  & 20 \\
JPM - WMT & RT - TS & 0.82  & 0.82  & 0.87  & 0.82  & 0.53  & 20 \\
V - GOOG & TS - EM & 0.81  & 0.81  & 0.82  & 0.84  & 0.37  & 20 \\
INTC - GOOG & RT - EM & 0.81  & 0.81  & 0.81  & 0.82  & 0.41  & 20 \\
XOM - WMT & TS    & 0.80  & 0.88  & 0.76  & 0.91  & 0.14  & 20 \\
INTC - WMT & RT - TS & 0.80  & 0.80  & 0.80  & 0.80  & 0.55  & 20 \\
QCOM - GOOG & ET - EM & 0.79  & 0.83  & 0.81  & 0.78  & 0.69  & 20 \\
INTC - HD & RT    & 0.79  & 0.79  & 0.85  & 0.80  & 0.49  & 20 \\
INTC - QCOM & RT - ET & 0.77  & 0.78  & 0.78  & 0.78  & 0.45  & 10 \\
JNJ - WMT & RT - TS & 0.77  & 0.87  & 0.82  & 0.74  & 0.81  & 20 \\
XOM - V & TS    & 0.76  & 0.85  & 0.72  & 0.86  & 0.15  & 20 \\
INTC - MSFT & RT    & 0.76  & 0.76  & 0.76  & 0.75  & 0.56  & 20 \\
QCOM - PFE & ET - RT & 0.75  & 0.76  & 0.81  & 0.77  & 0.47  & 20 \\
JPM - GOOG & RT - EM & 0.75  & 0.81  & 0.86  & 0.73  & 0.65  & 20 \\
CVX - V & EM - TS & 0.75  & 0.75  & 0.75  & 0.75  & 0.47  & 20 \\
XOM - HD & TS - RT & 0.74  & 0.74  & 0.74  & 0.74  & 0.46  & 10 \\
QCOM - V & ET - TS & 0.73  & 0.74  & 0.73  & 0.75  & 0.35  & 20 \\
PFE - GOOG & RT - EM & 0.73  & 0.73  & 0.77  & 0.75  & 0.43  & 10 \\
JPM - MSFT & RT    & 0.73  & 0.79  & 0.77  & 0.71  & 0.69  & 20 \\
CVX - PFE & EM - RT & 0.72  & 0.77  & 0.81  & 0.71  & 0.60  & 20 \\
INTC - PFE & RT    & 0.72  & 0.75  & 0.73  & 0.83  & 0.21  & 20 \\
XOM - JNJ & TS - RT & 0.72  & 0.81  & 0.69  & 0.88  & 0.13  & 20 \\
JPM - V & RT - TS & 0.69  & 0.75  & 0.80  & 0.69  & 0.62  & 20 \\
JPM - HD & RT    & 0.69  & 0.73  & 0.74  & 0.69  & 0.59  & 20 \\
QCOM - XOM & ET - TS & 0.69  & 0.69  & 0.69  & 0.69  & 0.50  & 20 \\
QCOM - WMT & ET - TS & 0.68  & 0.73  & 0.68  & 0.68  & 0.31  & 10 \\
QCOM - JPM & ET - RT & 0.68  & 0.68  & 0.73  & 0.72  & 0.41  & 20 \\
XOM - MSFT & TS - RT & 0.68  & 0.71  & 0.68  & 0.68  & 0.37  & 20 \\
CVX - JPM & EM - RT & 0.68  & 0.75  & 0.68  & 0.68  & 0.74  & 20 \\
INTC - CVX & RT - EM & 0.68  & 0.69  & 0.71  & 0.69  & 0.50  & 10 \\
XOM - GOOG & TS - EM & 0.67  & 0.69  & 0.68  & 0.67  & 0.39  & 20 \\
JPM - PFE & RT    & 0.67  & 0.69  & 0.72  & 0.79  & 0.24  & 20 \\
QCOM - JNJ & ET - RT & 0.67  & 0.68  & 0.73  & 0.69  & 0.49  & 20 \\
INTC - JPM & RT    & 0.67  & 0.69  & 0.71  & 0.67  & 0.55  & 20 \\
INTC - JNJ & RT    & 0.67  & 0.73  & 0.74  & 0.66  & 0.62  & 20 \\
CVX - WMT & EM - TS & 0.67  & 0.68  & 0.66  & 0.67  & 0.37  & 20 \\
V - MSFT & TS - RT & 0.66  & 0.72  & 0.66  & 0.72  & 0.79  & 20 \\
QCOM - MSFT & ET - RT & 0.65  & 0.72  & 0.76  & 0.65  & 0.62  & 20 \\
WMT - MSFT & TS - RT & 0.65  & 0.65  & 0.65  & 0.65  & 0.55  & 20 \\
INTC - V & RT - TS & 0.64  & 0.74  & 0.64  & 0.65  & 0.77  & 20 \\
JNJ - GOOG & RT - EM & 0.64  & 0.66  & 0.67  & 0.64  & 0.54  & 10 \\
CVX - JNJ & EM - RT & 0.63  & 0.63  & 0.69  & 0.69  & 0.35  & 20 \\
INTC - XOM & RT - TS & 0.62  & 0.68  & 0.63  & 0.71  & 0.20  & 20 \\
PFE - MSFT & RT    & 0.62  & 0.64  & 0.66  & 0.71  & 0.25  & 10 \\
PFE - WMT & RT - TS & 0.62  & 0.87  & 0.59  & 0.75  & 0.05  & 10 \\
V - HD & TS - RT & 0.60  & 0.61  & 0.60  & 0.60  & 0.58  & 20 \\
JNJ - HD & RT    & 0.60  & 0.64  & 0.60  & 0.60  & 0.67  & 10 \\
V - PFE & TS - RT & 0.60  & 0.78  & 0.60  & 0.88  & 0.06  & 20 \\
HD - WMT & RT - TS & 0.59  & 0.59  & 0.59  & 0.59  & 0.42  & 20 \\
XOM - PFE & TS - RT & 0.57  & 0.63  & 0.58  & 0.57  & 0.63  & 10 \\
JPM - JNJ & RT    & 0.56  & 0.63  & 0.59  & 0.57  & 0.62  & 10 \\
V - WMT & TS    & 0.56  & 0.87  & 0.58  & 0.55  & 0.91  & 20 \\
QCOM - HD & ET - RT & 0.56  & 0.59  & 0.61  & 0.58  & 0.51  & 10 \\
JNJ - MSFT & RT    & 0.54  & 0.81  & 0.54  & 0.55  & 0.90  & 20 \\
HD - GOOG & RT - EM & 0.53  & 0.63  & 0.56  & 0.54  & 0.65  & 10 \\
HD - MSFT & RT    & 0.52  & 0.85  & 0.52  & 0.53  & 0.92  & 10 \\
JNJ - PFE & RT    & 0.51  & 0.61  & 0.58  & 0.75  & 0.10  & 20 \\
V - JNJ & TS - RT & 0.50  & 0.86  & 0.50  & 0.50  & 0.94  & 10 \\
XOM - CVX & TS - EM & 0.49  & 0.52  & 0.54  & 0.56  & 0.22  & 10 \\
MSFT - GOOG & RT - EM & 0.48  & 0.94  & 0.47  & 0.50  & 0.94  & 20 \\
PFE - HD & RT    & 0.44  & 0.44  & 0.61  & 0.62  & 0.22  & 20 \\
\bottomrule
\label{Table:results_all_pairs_full}
\end{longtable}
\end{small}
